# Supplementary material for: Electrostatic Conveyer for Excitons
Source: arXiv:1102.5329 ancillary file (2011-02-25)
Supplement: Supplementary file 1 [file conveyer_supplementary_materials.pdf]

# Electrostatic Conveyer for Excitons
# Supplementary Materials

A. G. Winbow, J. R. Leonard, M. Remeika, Y. Y. Kuznetsova, A. A. High, A. T. Hammack, L. V. Butov
*Department of Physics, University of California at San Diego, La Jolla, CA 92093-0319, USA*

J. Wilkes, A. A. Guenther, A. L. Ivanov
*Department of Physics and Astronomy, Cardiff University, Cardiff CF24 3AA, United Kingdom*

M. Hanson, A.C. Gossard
*Materials Department, University of California at Santa Barbara, Santa Barbara, California 93106-5050*

(Dated: February 25, 2011)

PACS numbers:

**Circuit schematic of the conveyer RF system**

Figure S1 presents photographs of the lower part of the insert Octopus for optics and RF electronics at cryogenic temperatures. The Octopus has 8 broadband transmission lines providing up to 8 independent channels. Both the sample and electronic circuit on PCB next to the sample are in superfluid He in the conveyer experiment.

AC voltages to the conveyer electrodes on the sample are delivered via 7 broadband transmission lines with impedance-matching termination at the sample. We used coaxial cables UT-141B-SS silver-plated beryllium copper inner conductor, PTFE Teflon dielectric, and stainless-steel outer shell with diameter 3.6 mm, having a room-temperature attenuation of 3 dB/m at 10 GHz. The cable bandwidth complies with the frequency used in the experiments ($f_{\text{conv}}$ = 50 – 450 MHz), while the cable composition reduces heat conductance to the sample. The DC bias $V_{\text{bias}}$ is supplied separately via regular wires. The transmission lines are capacitively terminated to block DC heating at the termination resistors. Circuit schematic for the conveyer RF system is presented in Fig. S2 for one of the channels and in Fig. S3 for the entire system with 7 channels. A sample resistance between the top and bottom exceeds 10 MΩ in the experiments.

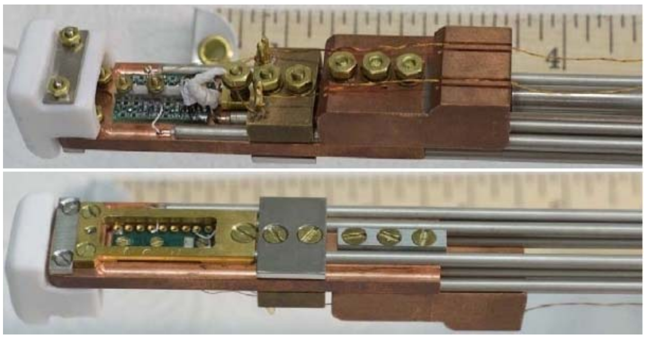

FIG. 1: Photographs of the lower part of the sample insert Octopus for optics and RF electronics at cryogenic temperatures from two sides. An electronic circuit on PCB is seen on the upper photo. A socket for a sample is seen on the lower photo. The ends of the ~ 1 m long transmission lines are on the right.

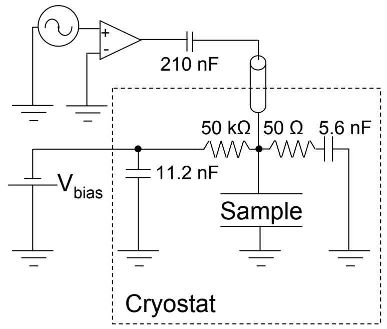


FIG. 2: Circuit schematic for one conveyer electrode line.

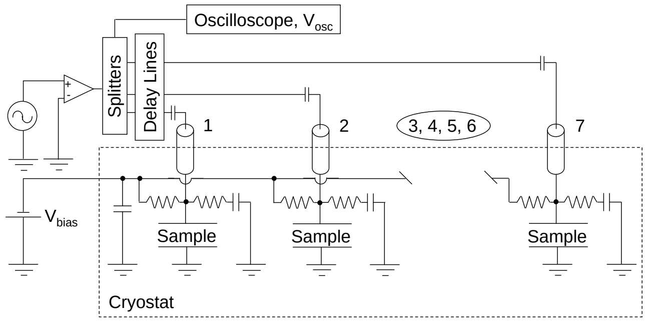


FIG. 3: Circuit schematic for the entire conveyer system with seven electrode lines.

**Calibration of the conveyer amplitude**

The conveyer amplitude is calibrated using the following procedure:

1. We applied AC voltage $V_{\text{osc}}$ to all conveyer electrodes in phase and measured the spectral linewidth of indirect excitons. The linewidth, characterized by the half width at half maximum HWHM, has a contri-

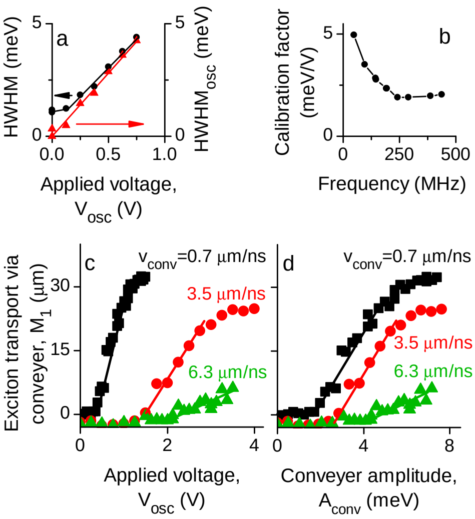


FIG. 4: Calibration of the conveyer amplitude. (a) AC voltage $V_{osc}$ is applied to all conveyer electrodes in phase. Spectral linewidth of indirect excitons HWHM at 50 MHz vs $V_{osc}$ (black points). The contribution from the energy oscillation of indirect excitons due to the oscillating voltage $HWHM_{osc} = [HWHM^2 - HWHM_0^2]^{1/2}$ vs $V_{osc}$ (red triangles). Red line with slope $m$ presents a linear fit with y-intercept fixed at 0. (b) The calibration curve for the conveyer amplitude: The ratio between the AC voltage supplied to the transmission lines at the top of the cryostat and the amplitude of energy oscillation of indirect excitons obtained from the simulations to fit the measured value of $m$ vs driving frequency. (c,d) The average transport distance of indirect excitons via conveyer $M_1$ vs (c) the applied AC voltage at the top of the cryostat and (d) the conveyer amplitude.

bution from the intrinsic linewidth of indirect excitons $HWHM_0$, which is present at zero voltage oscillation, and a contribution from the energy oscillation of indirect excitons $HWHM_{osc}$ due to the oscillating voltage. A defocused laser excitation with a spot ~ 50$\mu$m in diameter and $P_{ex}$ = 220$\mu$W was used. Figure S4a presents the measured HWHM as a function $V_{osc}$ for one of the frequencies.

2. We subtracted in quadrature $HWHM_0$ from HWHM to obtain $HWHM_{osc}$ (Fig. S4a).

3. We performed numerical simulations of $HWHM_{osc}$ vs the amplitude of exciton energy oscillation. The comparison of these simulations to the experimental data allows to determine the amplitude of exciton energy oscillation. Figure S4c presents the obtained ratio between the AC voltage supplied to the transmission lines at the top of the cryostat $V_{osc}$ and the amplitude of energy oscillation of indirect excitons $A_{conv}$ as a function of frequency. This is the calibration curve for the conveyer amplitude. Figure S4c and S4d show the average transport distance of indirect excitons via conveyer $M_1$ as a function of $V_{osc}$ and $A_{conv}$, respectively.

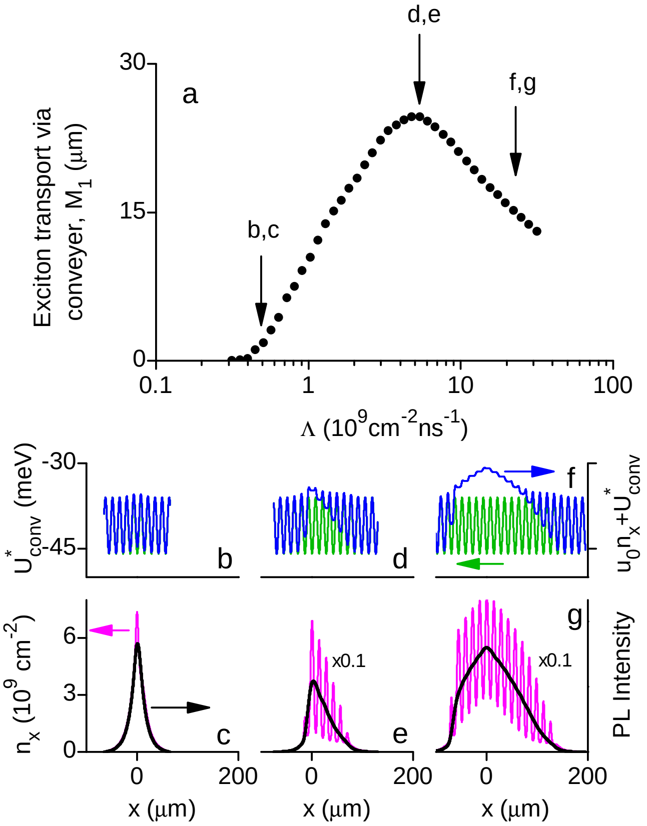


FIG. 5: (a) Calculated average transport distance of indirect excitons via conveyer $M_1$ as a function of exciton generation rate. (b-g) A snapshot of the conveyer potential $U^*_{conv}$ (green), exciton density distribution (magenta), and corresponding screened conveyer potential (blue). Time-integrated PL intensity (black). $\Lambda = 0.51 \cdot 10^9$ (b,c), $5.4 \cdot 10^9$ (d,e), and $22 \cdot 10^9 cm^{-2}ns^{-1}$ (f,g). $A_{conv}$ = 4.9 meV, $v_{conv}$ = 0.7$\mu$m/ns.

**Simulation details**

Figure S5 presents details of the simulations for the density dependence of exciton transport via conveyer. In these simulations, the conveyer potential is approximated by a cosine function and the effect of the disorder and conveyer ripples on exciton transport is approximated within the thermionic model via the modification of the exciton diffusion coefficient as described in the main text. Attached movie "density dependence" presents more details of the simulations keeping the format of Fig. S5b-g.

Another attached movie "conveyer amplitude dependence" presents details of the simulations for the conveyer amplitude dependence of exciton transport via conveyer (Fig. 4a,b) keeping the format of Fig. 4a,b.
